# Supplementary material for: An exact analytical scheme using a new potential to solve one-dimensional quantum systems
Source: arXiv:1805.01895 source file (2020-03-09)

# Mathematica code for solving time-independent Schrodinger equation

The Mathematica code is presented that can solve the Schrodinger equation for arbitrary potential function $V(x)$ and effective mass function $m(x)$ given as the inputs. The code returns the transmission probability, energy eigenvalues, energy eigenfunctions. The code should be optimized for getting higher accuracies. The pseudo-codes presented at the appropriate places can help in using the code.The solver calculates the transmission probability,eigenvalues and the eigenfunctions for the problem.

Note: You can contact the corresponding author to check if there is an update available for the code.

In[ ]:=
```
Unprotect["Global`*"];
Remove["Global`*"];
ClearAll["Global`*"];
n = 9;(*Give n as 2i+
 1 where `i' is the number of ultrashort barriers in the collection*)
Tn[-1] = IdentityMatrix[2];
For[o = 0, o ≤ (n - 3) / 2, o++,
  Print[Tn[o] = Simplify[Tn[o - 1].Inverse[A[a2 o+1, Vo*2+1]].Em[a2 o+1, V2 o+1]]]];
 (*Transfer matrix mulitplications*)
A[a1_, Vj_] :=
  {{Exp[I * kj * a1], Exp[-I * kj * a1]}, {-I * kj * Exp[I * kj * a1], I * kj * Exp[-I * kj * a1]}};
 (*Matrices for scattering states*)
Em[a1_, Vj_] := {{Exp[I * kj+2 * a1+1], Exp[-I * kj+2 * a1+1]},
   {-I * kj+2 * Exp[I * kj+2 * a1+1] - 2 mj+1 / ℏ^2 (En - Vj+1) (a1+1 - a1) Exp[I * kj+2 * a1+1],
    I * kj+2 * Exp[-I * kj+2 * a1+1] - 2 mj+1 / ℏ^2 (En - Vj+1) (a1+1 - a1) Exp[-I * kj+2 * a1+1]}};
Print["The transmission coefficient is given by"];
Tn[(n - 3) / 2];
T[En_] = Assuming[Element["Global`*", Reals], Abs[%[[1, 1]]]^2];(*T(En)= t11*)
kj_ := Sqrt[2 mj / ℏ^2 * (En - Vj)];
Print["The bound state equation is given by"];
Tn[(n - 3) / 2] /. {Vj_ → Vm - Vj};
Tb[En_] = Assuming[Element["Global`*", Reals], %[[1, 1]]];
(*eigen energies are obtained from zeros of this function*)
r = 0.8400934725278035`;(*SeedRandom[2345];RandomReal[]*)
T[(n + 1)/2] = {r, -r};
For[o = (n + 1) / 2, o ≥ 2, o--,
  Print[T[o - 1] = Simplify[Inverse[A1[ao, Vo]].Em1[ao, Vo].T[o]]]];
A1[a1_, Vj_] := {{Cosh[κ2 j-3 * a2 1-3], (HeavisideTheta[(Vm - V2 j-3) - En] -
       I * HeavisideTheta[-(Vm - V2 j-3) + En]) * Sinh[κ2 j-3 * a2 1-3]},
   {-κ2 j-3 (HeavisideTheta[(Vm - V2 j-3) - En] + I * HeavisideTheta[-(Vm - V2 j-3) + En]) *
     Sinh[κ2 j-3 * a2 1-3] *
     (HeavisideTheta[(Vm - V2 j-3) - En] - I * HeavisideTheta[-(Vm - V2 j-3) + En]),
```

Printed by Wolfram Mathematica Student Edition

```
    -κ_{2 j-3} (HeavisideTheta[(Vm - V_{2 j-3}) - En] - I * HeavisideTheta[-(Vm - V_{2 j-3}) + En]) *
     Cosh[κ_{2 j-3} * a_{2 l-3}]}};
Em1[a1_, Vj_] := {{Cosh[κ_{2 j-1} * a_{2 l-2}], (HeavisideTheta[Vm - V_{2 j-1} - En] -
       I * HeavisideTheta[-(Vm - V_{2 j-1}) + En]) * Sinh[κ_{2 j-1} * a_{2 l-2}]},
   {-κ_{2 j-1} * (HeavisideTheta[(Vm - V_{2 j-1}) - En] + I * HeavisideTheta[-(Vm - V_{2 j-1}) + En]) *
      (HeavisideTheta[(Vm - V_{2 j-1}) - En] - I * HeavisideTheta[-(Vm - V_{2 j-1}) + En]) *
      Sinh[κ_{2 j-1} * a_{2 l-2}] - 2 m_{2 j-2} / ħ^2 (En - (Vm - V_{2 j-2})) (a_{2 l-2} - a_{2 l-3}) Cosh[κ_{2 j-1} * a_{2 l-2}],
    -κ_{2 j-1} (HeavisideTheta[(Vm - V_{2 j-1}) - En] - I * HeavisideTheta[-(Vm - V_{2 j-1}) + En]) *
      Cosh[κ_{2 j-1} * a_{2 l-2}] - 2 m_{2 j-2} / ħ^2 (En - (Vm - V_{2 j-2})) (a_{2 l-2} - a_{2 l-3})
      (HeavisideTheta[(Vm - V_{2 j-1}) - En] - I * HeavisideTheta[-(Vm - V_{2 j-1}) + En]) *
      Sinh[κ_{2 j-1} * a_{2 l-2}]}};
Print["The coefficients given by"]
ss1 = T[1];
ψ[x_] =
  Sum[HeavisideTheta[x - a_{2 j+1}] HeavisideTheta[-x + a_{2 j+2}] * (T[j + 2][[1]] * Cosh[κ_{2 j+3} a_{2 j+2}] +
       T[j + 2][[2]] * (HeavisideTheta[Vm - V_{2 j+3} - En] - I * HeavisideTheta[-(Vm - V_{2 j+3}) + En])
        Sinh[κ_{2 j+3} a_{2 j+2}]), {j, 0, (n - 3)/2}] +
   Sum[HeavisideTheta[x - a_{2 j}] HeavisideTheta[-x + a_{2 j+1}] *
     (T[j + 1][[1]] * Cosh[κ_{2 j+1} x] + T[j + 1][[2]] * (HeavisideTheta[(Vm - V_{2 j+1}) - En] -
          I * HeavisideTheta[-(Vm - V_{2 j+1}) + En]) Sinh[κ_{2 j+1} x]), {j, 1, (n - 3)/2}] +
   HeavisideTheta[a_1 - x] (T[1][[1]] * Cosh[κ_1 x] + Sinh[κ_1 x] * T[1][[2]]) +
   HeavisideTheta[x - a_{n-1}]
    (T[(n + 1)/2][[1]] Cosh[κ_n x] + T[(n + 1)/2][[2]] Sinh[κ_n x]);(*wavefunction*)
ψ[x];
κ_{j_} := Sqrt[2 m_j / ħ^2 * (-En + Vm - V_j)];
ħ = 1;
a_1 = -1.525;(*Initial point of the barrier*)
For[i = 1, i ≤ n, i++, Print[a_{2 i+1} = a_1 + 1 * i]];
(*relative distance between the barriers*)
For[i = 1, i ≤ n, i++, Print[a_{2 i} = a_{2 i-1} + .05]];(*Width of the ultrashort barrier*)
m[x_] = 1;(*1*Sqrt[7/π]*Exp[-7*(x-a_{(n-1)/2})^2]*)
For[i = 1, i ≤ n + 4, i++, Print[m_i = m[(a_{i-1} + a_i)/2]]];
(*If you have defined position-dependent mass function as m[x] give m_i as m_i=m[(a_{i-1}+a_i)/2]*)
V[x_] = 20 * UnitStep[x + 1.525] * UnitStep[1.525 - x];
(*1*Sqrt[7/π]*Exp[-7*(x-a_{(n-1)/2})^2]*)
For[i = 2, i ≤ n - 1, i++, Print[V_i = V[(a_{i-1} + a_i)/2]]];
(*Potential value between the break points a_{i-1}-
 a_i. For any other potential fucntion(V[x]) replace V_i as, V_i=V[(a_{i-1}+a_i)/2]*)
V_1 = 0;(*Asymptotic potentials V1 and Vn*)
V_n = 0;
Vm = Max[Table[V_i, {i, 1, n}]];
(*PlotLegends position paramters*)
h = -.4;
```

```
y = -1.7;
ys = 0;
p1t = Plot[1/T[En], {En, 0, Vm + 4},
   PlotLegends → Placed[{Style[(n - 1) / 2 "UB", 13]}, {Scaled[{0, 0.5}], {y - 0.7, h - 2}}],
   PlotRange → {-0.07, 1.03}, PlotTheme → {"Scientific", "Monochrome"},
   PlotLabel → {Style["Transmission probability versus energy", 14]},
   FrameLabel → {Style["E ", 14], Style["T(E)", 14]}, PlotStyle → {Dashed}];
f1 = En /. NSolve[Tb[En] == 0 && En > 0 && En ≤ V_((n+1)/2), En, WorkingPrecision → 10,
    VerifySolutions → True, RandomSeeding → 1234];
If[Thread[Table[Tb[En] /. En → f1[[l]], {l, 1, Length[f1]}] ≤ 10^-12] ==
   Table[True, {l, 1, Length[f1]}], Print["Obtained energy values are bound states"],
  Print["Energy values are erraneous"]];
e = Input[Print["The well has" Length[f1]
     "bound states, please enter the node of the state"]];
Print["THe corresponding energy value"]
En = f1[[e + 1]] (*f[[e]];*)
Print["The wavefunction becomes"]
ψ[x];
A1 = NIntegrate[Abs[ψ[x]]^2, {x, -30, 30}];
(*PlotLegends position parameters*)
h = -.4;
y = -1.7;
ys = 0;
Print["The amplitude on the left and
   right is compared between exponential and cosh, Sinh basis"]
ss1
{r, -r}
p1w = Plot[Simplify[ψ[x] / √A1], {x, -a_(n-1) - 4, a_(n-1) + 4},
   PlotLegends → Placed[{Style[(n - 1) / 2 "UW", 13]}, {Scaled[{0, 0.5}], {y - 0.7, h - 2}}],
   PlotTheme → {"Scientific", "Monochrome"}, PlotLabel → {Style["Eigenfunction" ψ_e, 14]},
   FrameLabel → {Style["x ", 14], Style["Wavefunction ψ[x]", 14]}, PlotStyle → {Dashed}];
V0 = V_((n+1)/2);
Print["The d is"]
d = (a_(n-1) - a_1);
ma = 1;
k2 = Sqrt[2 ma * (En1 - (Vm - V_((n+1)/2))) / ℏ^2];
k1 = Sqrt[2 ma * (Vm - V_n - En1) / ℏ^2];
s = d / 2;
k3 = Sqrt[2 ma * (-En + Vm - V_n) / ℏ^2];
k4 = Sqrt[2 ma * (-(Vm - V_((n+1)/2)) + En) / ℏ^2]
Tconw[En1_] = Cos[k2 * d] + 1/2 Sin[k2 * d] (k1/k2 - k2/k1);
Clear[En]
Tconb[Enr_] =
  1 / (1 + 1 / 4 * V0^2 / ((Enr - V0) Enr) * (Sin[d * Sqrt[2 * ma (Enr - V0) / ℏ^2]])^2);
p2t = Plot[Tconb[Enr], {Enr, 0, Vm + 4},
  PlotLegends → Placed[{Style["Rectangle", 13]}, {Scaled[{0, 0.5}], {y, h - 1}}],
```

```
  PlotRange → {-0.07, 1.03}, PlotTheme → {"Scientific", "Monochrome"},
  PlotLabel → {Style["Transmission probability versus energy", 14]},
  FrameLabel → {Style["E ", 14], Style["T(E)", 14]}, PlotStyle → {Gray}]
f2 = En1 /. NSolve[Cos[4.31335136523794` Sqrt[En1]] +
     1/2 (Sqrt[20 - En1]/Sqrt[En1] - Sqrt[En1]/Sqrt[20 - En1]) Sin[4.31335136523794` Sqrt[En1]] == 0 && En1 > 0 && En1 ≤ V0,
   En1, WorkingPrecision → 10, VerifySolutions → True, RandomSeeding → 1234]
   (*Transmission of the rectangular function*)
ϕ[x_] = Piecewise[{{2 * B * Cos[k4 * s] * Exp[k3 * (x + s)], x < -s},
    {2 * B * Cos[k4 * x], s > x > -s}, {2 * B * Cos[k4 * s] * Exp[-k3 * (x - s)], s < x}}];
{B, B1} = B /. Solve[Integrate[ϕ[x]^2, {x, -∞, ∞}] == 1, B];
p2w = Plot[ϕ[x], {x, -s - 4, s + 4},
  PlotLegends → Placed[{Style["Rectangle", 13]}, {Scaled[{0, 0.5}], {y, h - 1}}],
  PlotRange → {-1, 1}, PlotTheme → {"Scientific", "Monochrome"},
  PlotLabel → {Style["Eigenfunction" ψn-2, 14]},
  FrameLabel → {Style["position ", 14], Style["ψ(x)", 14]}, PlotStyle → {Gray}]
Show[p2t, p1t]
Print["Eigenvalues using ultrashort well"]
f1
Print["Eigenvalues of the rectangular well"]
f2
Print["The transmission coefficient is given by"]
Show[p1w, p2w]
```

$\{\{1, 0\}, \{0, 1\}\}.Inverse[A[a_1, V_1]].Em[a_1, V_1]$

$\{\{1, 0\}, \{0, 1\}\}.Inverse[A[a_1, V_1]].Em[a_1, V_1].Inverse[A[a_3, V_3]].Em[a_3, V_3]$

$\{\{1, 0\}, \{0, 1\}\}.Inverse[A[a_1, V_1]].Em[a_1, V_1].Inverse[A[a_3, V_3]].Em[a_3, V_3].Inverse[A[a_5, V_5]].Em[a_5, V_5]$

$\{\{1, 0\}, \{0, 1\}\}.Inverse[A[a_1, V_1]].Em[a_1, V_1].Inverse[A[a_3, V_3]].Em[a_3, V_3].Inverse[A[a_5, V_5]].Em[a_5, V_5].Inverse[A[a_7, V_7]].Em[a_7, V_7]$

The transmission coefficient is given by

The bound state equation is given by

$Inverse[A1[a_5, V_5]].Em1[a_5, V_5].\{0.840093, -0.840093\}$

$Inverse[A1[a_4, V_4]].Em1[a_4, V_4].Inverse[A1[a_5, V_5]].Em1[a_5, V_5].\{0.840093, -0.840093\}$

$Inverse[A1[a_3, V_3]].Em1[a_3, V_3].Inverse[A1[a_4, V_4]].Em1[a_4, V_4].Inverse[A1[a_5, V_5]].Em1[a_5, V_5].\{0.840093, -0.840093\}$

$Inverse[A1[a_2, V_2]].Em1[a_2, V_2].Inverse[A1[a_3, V_3]].Em1[a_3, V_3].Inverse[A1[a_4, V_4]].Em1[a_4, V_4].Inverse[A1[a_5, V_5]].Em1[a_5, V_5].\{0.840093, -0.840093\}$

The coefficients given by

-0.525

0.475

1.475

2.475

3.475

4.475

5.475

6.475

7.475

−1.475

−0.475

0.525

1.525

2.525

3.525

4.525

5.525

6.525

1

1

1

1

1

1

1

1

1

1

1

1

1

20

20

20

20

20

20

20

Obtained energy values are bound states

7 bound states, please enter the node of the state The well has

THe corresponding energy value

Out[ ]= 19.65582400

The wavefunction becomes

NIntegrate: NIntegrate failed to converge to prescribed accuracy after 9 recursive bisections in x near {x} = {0.585005}. NIntegrate obtained 0.15740159587172597` and 0.000016365500381570095` for the integral and error estimates.

The amplitude on the left and right is compared between exponential and cosh, Sinh basis

Out[ ]= {0.840093 + 0. i, 0.840093 + 0. i}

Out[ ]= {0.840093, -0.840093}

The d is

Out[ ]= 6.269900159

Out[ ]=

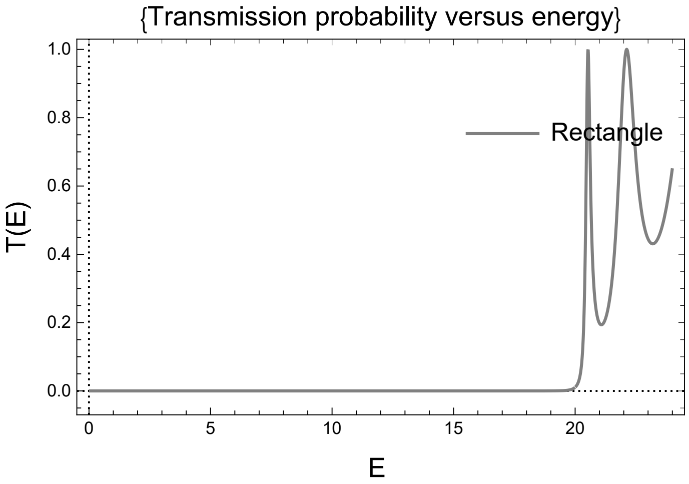


Out[ ]= {0.4351950532, 1.737055797, 3.893317759, 6.878983421, 10.64446179, 15.07385175, 19.64370439}

Out[ ]=

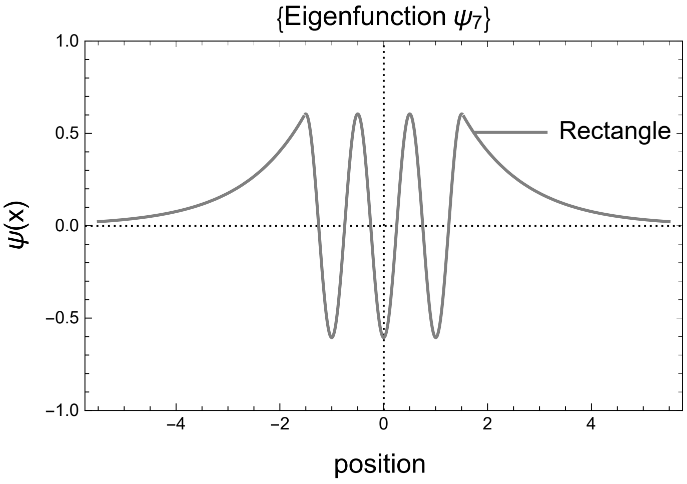

Out[ ]=

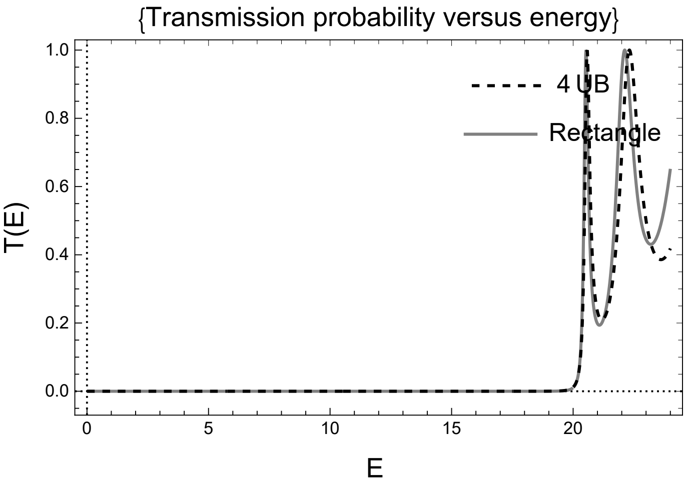


Eigenvalues using ultrashort well

Out[ ]= {0.4675977790, 1.871995241, 4.324177294, 7.169339934, 11.22567835, 15.86817433, 19.65582400}

Eigenvalues of the rectangular well

Out[ ]= {0.4351950532, 1.737055797, 3.893317759, 6.878983421, 10.64446179, 15.07385175, 19.64370439}

The transmission coefficient is given by

Out[ ]=

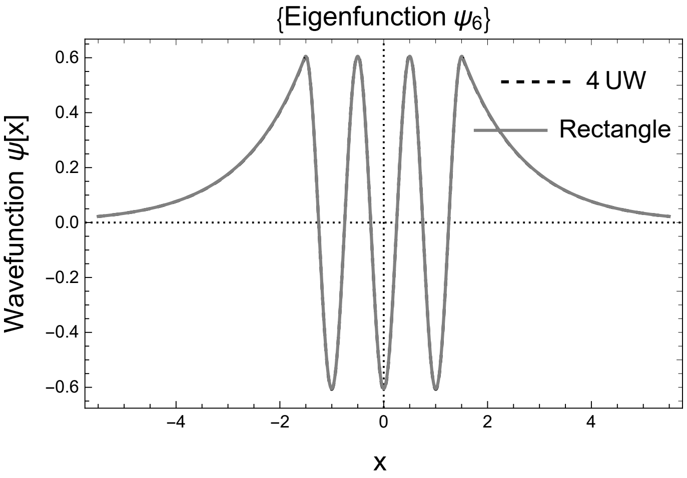

Supplement: Supplementary file 1 [file ultrashortv7supplementaru.pdf]
